# Supplementary material for: Preserving Distances in Very Faulty Graphs
Source: arXiv:1703.10293 source file (2017-03-30)
Supplement: Supplementary file 2 [file AppendixTablesFigures.tex]

\newpage
\section{Tables}
\label{sec:tabFig}

\begin{tabular}{ |c|c|c|c| }
%\begin{center}
\hline
\multicolumn{4}{ |c| }{$f$-VFT (or EFT) Preservers} \\
\hline
& \shortstack{$S$-sourcewise \\(unweighted)} & \shortstack{pairs $P$, $f=1$ \\ (weighted)} & \shortstack{Single pair $s$-$t$, $f=1$\\(weighted+directed)} \\ \hline
\multirow{2}{*}{\shortstack{Upper \\ Bound}} & $\widetilde{O}(f|S|^{1/2^f} \cdot n^{2-1/2^f})$ & $O(\min\{n^2,n|P|\})$ & $O(DP(n))=O(n^{3/2})$\\
 & \mbox{\textbf{New}} & \mbox{\textbf{New}} 
 & \mbox{\textbf{New}} \\ \hline
\multirow{2}{*}{\shortstack{Lower \\ Bound}} & $\Omega(|S|^{1/(f+1)} \cdot n^{2-1/(f+1)})$ & $\Omega(\min\{n^2,n|P|\})$ & $\Omega(DP(n))=\Omega(n^{4/3})$ \\
 & \cite{ParterPODC15} & \mbox{\textbf{New}} & \mbox{\textbf{New}}\\
\hline
%\end{center}
\end{tabular}
